# Supplementary material for: Addressing UX Practitioners' Challenges in Designing ML Applications: an Interactive Machine Learning Approach
Source: arXiv:2302.11843 source file (2023-02-23)
Supplement: Supplementary file 1 [file appendix.tex]

\section{Interview Protocol}
\subsection*{Introduction and preliminaries}
Hello, how are you? [other intro pleasantries]

I’m Kevin, a PhD student in the department of Human Centered Design \& Engineering at the University of Washington. Today, we’re asking you to participate in an activity where you will design a proof-of-concept app that uses machine learning and construct a short design pitch for the app. The entire activity is estimated to take around 2 hours. We estimate that about an hour and 30 minutes will be spent on the app and its pitch, and about 30 minutes will be a follow-up interview. The pitch consists of only slides and you do not need to give a presentation to me. 

Do you have any questions before we get started?

Do I have your permission to record this Zoom session? We are interested in having an audio so that we can have an accurate transcript.

May I also turn on the automatic transcription in Zoom? This will speed our transcription efforts by providing an initial rough transcript of this session.

We will start the audio recording during the interview portion of this activity, which will take place later.

I’m going to first send you a link to a zip file with the files we’ll need for this activity. 

[link]

Go ahead and download and unzip the file. After you complete the study, feel free to delete the files. If you navigate into the unzipped folder, you should see two sub-folders: tutorial and activity. Do you see them? 

\subsection*{Tutorial}

Before we get started on the actual activity, I’m going to walk you through a quick tutorial of the machine learning tool we’ll be using. That’s where the tutorial folder you just downloaded comes handy. If you’re comfortable with screen sharing, I’ll just ask you to do that so I can help you better walk through the steps. Before you share, please make sure you don’t have any sensitive information on your screen.

Go into the tutorial folder, then go into the train folder, and let me know if you see 3 folders: husky, samoyed, corgi. Do they contain images of dogs inside? Good, I’ll send you a link to the actual tool now:

\url{https://teachablemachine.withgoogle.com/}

Once you’re on the site, click Get Started, then Image Project, then Standard image model. Ok, do you see a screen with “class 1, class 2, training, and preview”? Great.

We’re going to start with something called binary classification, so this machine learning model you’re going to train will distinguish images belonging to two classes. You can think of classes as categories for images. For example, our model will be able to differentiate huskies and samoyeds.

Now we’re ready to upload the husky images from the training folder to class 1. In the class 1 module, click Upload. Go into the husky folder (in the train folder), select all images, and drag them all into class 1.  Do you see 20 images of huskies in Class 1? Now let’s rename the class to Husky by clicking on the pencil icon next to the title.

Now we’re going to do the same thing for samoyeds and class 2. So click upload, go into the samoyed folder and drag them onto class 2 and rename the class to be samoyed.

Great, we’re ready to train the model, so click Train Model, and wait for it to finish. There are also some options under the Advanced tab in the training module that you’re free to explore later on in the main activity.

Ok, we’ve just trained a machine learning model, we can see if it works. We won’t be using the webcam to test, so click on the webcam dropdown (in the Preview module) and change that to file. Now you can go to the test folder instead of the train folder (that you just downloaded). You can drag images in one at a time to the Preview module and see how the classifier does. Right now, just test with images h0, h1, s0, and s1.

Great, now we’re ready to move on to something a bit more complicated: we’re going to add one more class and retrain the model. So click Add a class on the left, then upload. Navigate to the train folder again, and then select corgi. Select all the images and drag them into the new class. Rename that class Corgi. Now just click Train Model again. 

The model’s finished training, so we can test using all the images in our test folder.  Now you can go to the test folder and drag the images one by one into Preview. How does the model do?

Do you think you have a good idea of how to use this tool to train an image-based machine learning model? Do you have any questions at this point?

\subsection*{Design Activity}
Great. Now that you’re familiar with Teachable Machine, let’s move on to the main activity. 
Head into the activity folder (which you downloaded). Inside, you should see a datasets folder and a pdf called “instructions”. Do you see it?

Open up the instructions; this has all the info you’ll need to complete this activity. On page 2, there’s the design prompt. I’ll just review that with you quickly to set the stage for what’s to come:

Your company likes to invest in new ideas, particularly ones that use machine learning. You and another designer have an idea for a mobile app that uses machine learning to help users eat better. Since everyone loves taking photos of their food, your idea is to automatically categorize food photos as part of a photographic food journal. Your task is to design and present a proof-of-concept for the app, but you only need to focus on the part where the app automatically classifies food photos with machine learning since the other designer’s working on the journal experience. The deliverable is a pitch with 10 slides/pages or less. These are only slides, and you don’t need to give a presentation.

On page 3, you have some user research insights to help you get started. On page 4, there’s a persona based off of those insights. On page 5, there’s a description of what’s inside the datasets folder, which contains images for you to train image models. I’ll just point out that there are 3 different datasets that can be turned into 3 different models, each one with different behaviours. To help you navigate that folder, you can refer to the file structure diagram. On pages 6 and 7, there’s a food pyramid and descriptions of its contents, published by the US Department of Agriculture. On page 8, there’s a guide for you to create your design pitch at the end. 

To reiterate, if you just go back to page 5, the 3 subfolders in the train folder will lead to models with different UXs. We suggest that you train all 3 and pick what you think is best for the app to use for the rest of this activity. You can test the models with images in the test folder.

Overall, the UX of a machine learning based application can be quite different from traditional applications. As you work through this activity, you probably want to think about two specific challenges:
\begin{itemize}
    \item How to manage this different UX for the end user, and
    \item How you can effectively communicate the potential benefits and risks of this new app in your pitch
\end{itemize}

Ok, so the next hour and 15 mins are going to be work time for you. You can spend it any way you like. Here’s a recommended time allotment:
\begin{itemize}
    \item 30 minutes getting familiar with the instructions and training models with the data and picking one to use
    \item 45 minutes putting together the pitch and the materials you’ll need for it. By materials you’ll need, this is completely up to you, and can include things such as low fi wireframes, storyboards, sketches, or anything else you see fit. The pitch shouldn’t be longer than 10 slides.
\end{itemize}

Any questions? If not, I’ll leave you to it. I’ll be around, but I’ll turn off my camera and mute myself. Feel free to do the same and put on some music or whatever it is you like to do when working. You can also stop screen sharing. If you have any questions, you can unmute and say them—I’ll be here—or you can type it into the chat and I’ll respond there. I’ll also check in every once in a while. Sounds good? Ok, see you in a bit.

[checks in every 20 minutes or so]

\subsection*{Closing interview}
Ok, congratulations on completing the main activity! Now that you have your pitch, please export it as a PDF. Can you please email it to me? I’ve sent my email in the chat. Thanks, I got it.

Now, let’s move onto the interview portion of the study, where I’m going to ask you some questions about your experience just now. Before we start, do you consent to being audio recorded for this portion? No questions are mandatory, and you can revoke your consent at any time. 

Great. To start off, I’m curious to know, what got you started in UX?
Where did you do your training?

\subsubsection*{Calibration}
\begin{itemize}
    \item What expectations did you have for designing with AI in general before this activity?
    \item When does your team perform activities like this?
    \item Do you consider the app you just designed an effective use of AI for end users?
\end{itemize}

\subsubsection*{Tool} to be clear, this isn’t our tool, so you’re not going to hurt our feelings by critiquing it. It’s a tool that we picked among other similar tools that we think would be good for this activity.
\begin{itemize}
    \item How did the tool allow you to achieve the goals that you envisioned for the product?
    \item What was easy to use about the tool?
    \item What was not easy to use, or confusing, about this tool?
    \item Did this tool give you everything you need for you to put together your deliverable? If not, how could the tool have helped you out more?
    \item What do you think stakeholders want to see?
    \item How could the tool better support you in iterating your prototype with users?
    \item How could the tool better support you in understanding and exploring the machine learning models you trained?
    \item How could the tool better support you in explaining or communicating the machine learning models you trained to other people?
\end{itemize}

\subsubsection*{Pitch}

\begin{itemize}
    \item What did you use to create your pitch, both the slide deck and any assistive materials?
    \item In your pitch, you chose to use the ML model with [x] classes. Why did you make the choice of selecting this set of classes over the other 2 options?
    \item If you had the chance to organize your own set of classes from the data, what would that look like?
    \item What ethical challenges or risks do you think were the most important to communicate in your pitch?
    \item How might those be represented or made more obvious by the tool you used to train the models?
    \item Overall, we gave you an hour and 15 minutes to put this together. If you were given more time and resources, what would you do to improve your pitch?
\end{itemize}

Do you have any final questions or thoughts or anything else you would like me to know before we end?

Regarding the gratuity you’ll receive for this study, you should receive your \$40 Amazon gift card by email in [time]. Just to confirm, your preferred email is [email]? Thank you so much for your participation in this study! We hope it was a great experience. If you know anyone who is interested in participating, please encourage them to fill out our screener. Have a great day.

\section{Instructional PDF}

\begin{figure}[h]
    \begin{subfigure}[h]{0.49\textwidth}
        \centering
        \includegraphics[height=0.6\textwidth]{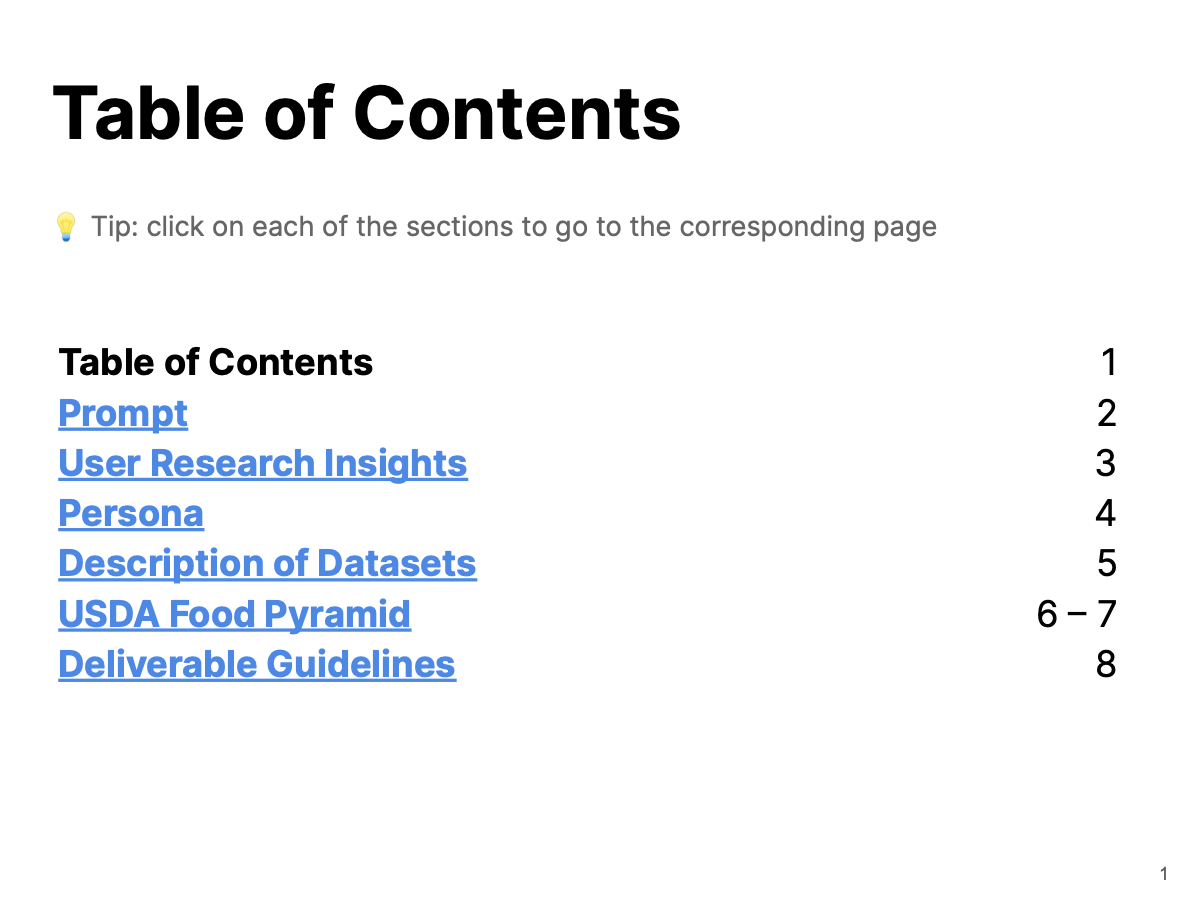}
    \end{subfigure}
    \begin{subfigure}[h]{0.49\textwidth}
        \centering
        \includegraphics[height=0.6\textwidth]{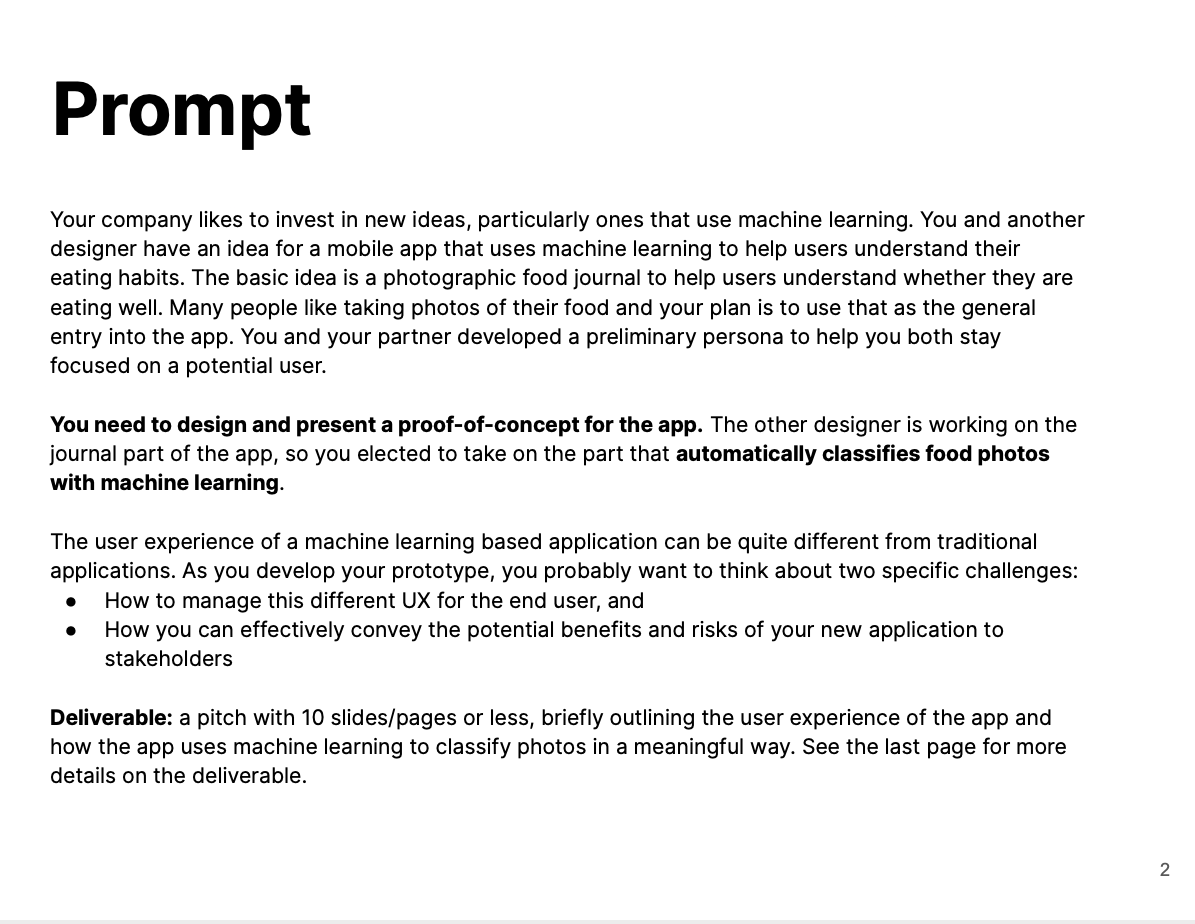}
    \end{subfigure}
    \begin{subfigure}[h]{0.49\textwidth}
        \centering
        \includegraphics[height=0.6\textwidth]{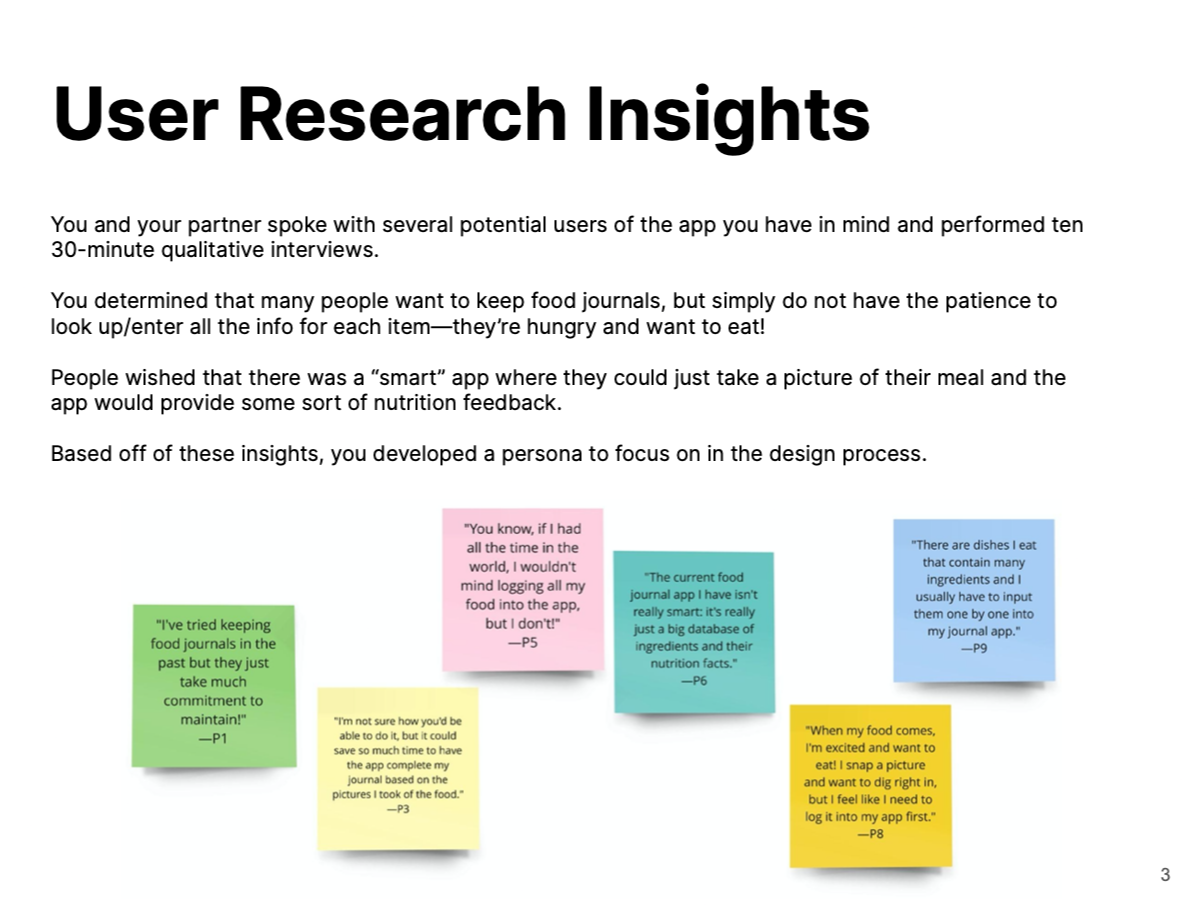}
    \end{subfigure}
    \begin{subfigure}[h]{0.49\textwidth}
        \centering
        \includegraphics[height=0.6\textwidth]{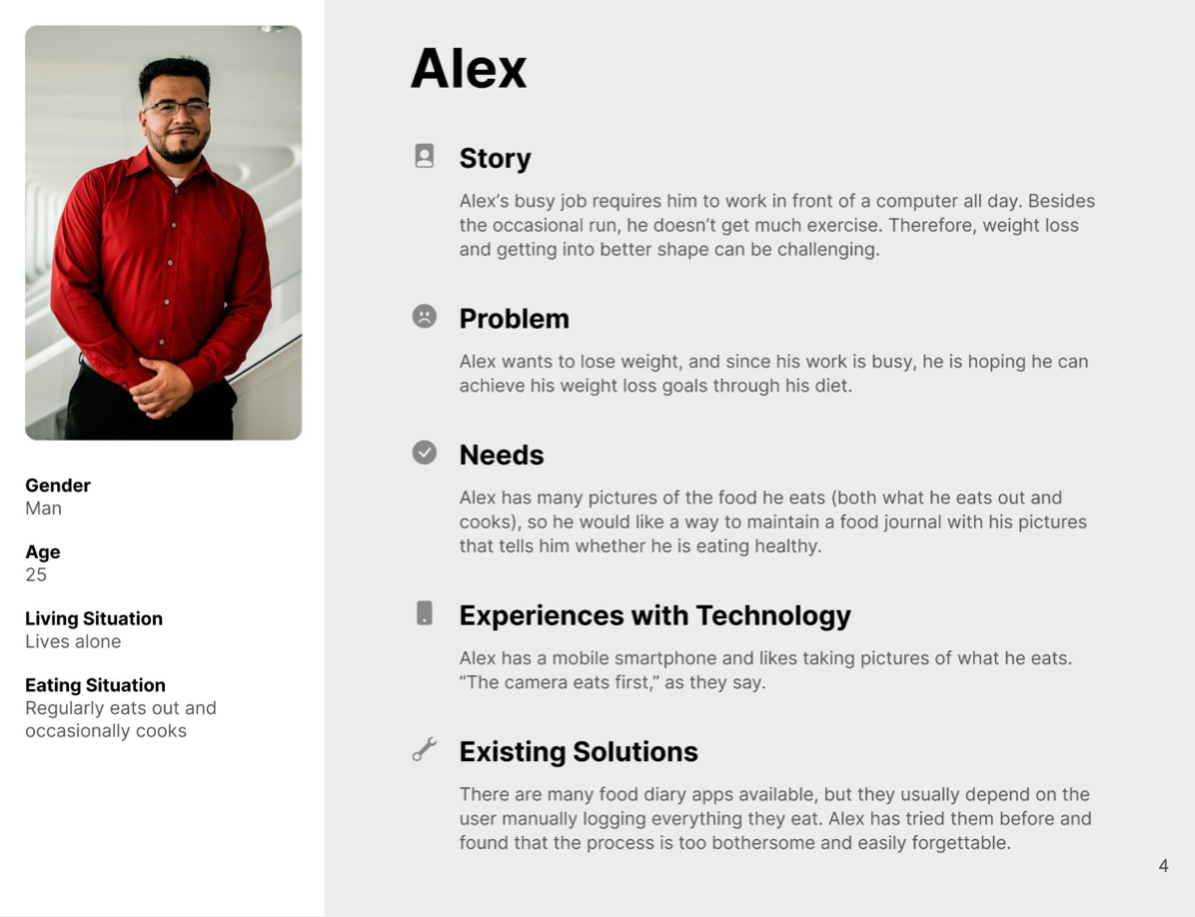}
    \end{subfigure}
    \begin{subfigure}[h]{0.49\textwidth}
        \centering
        \includegraphics[height=0.6\textwidth]{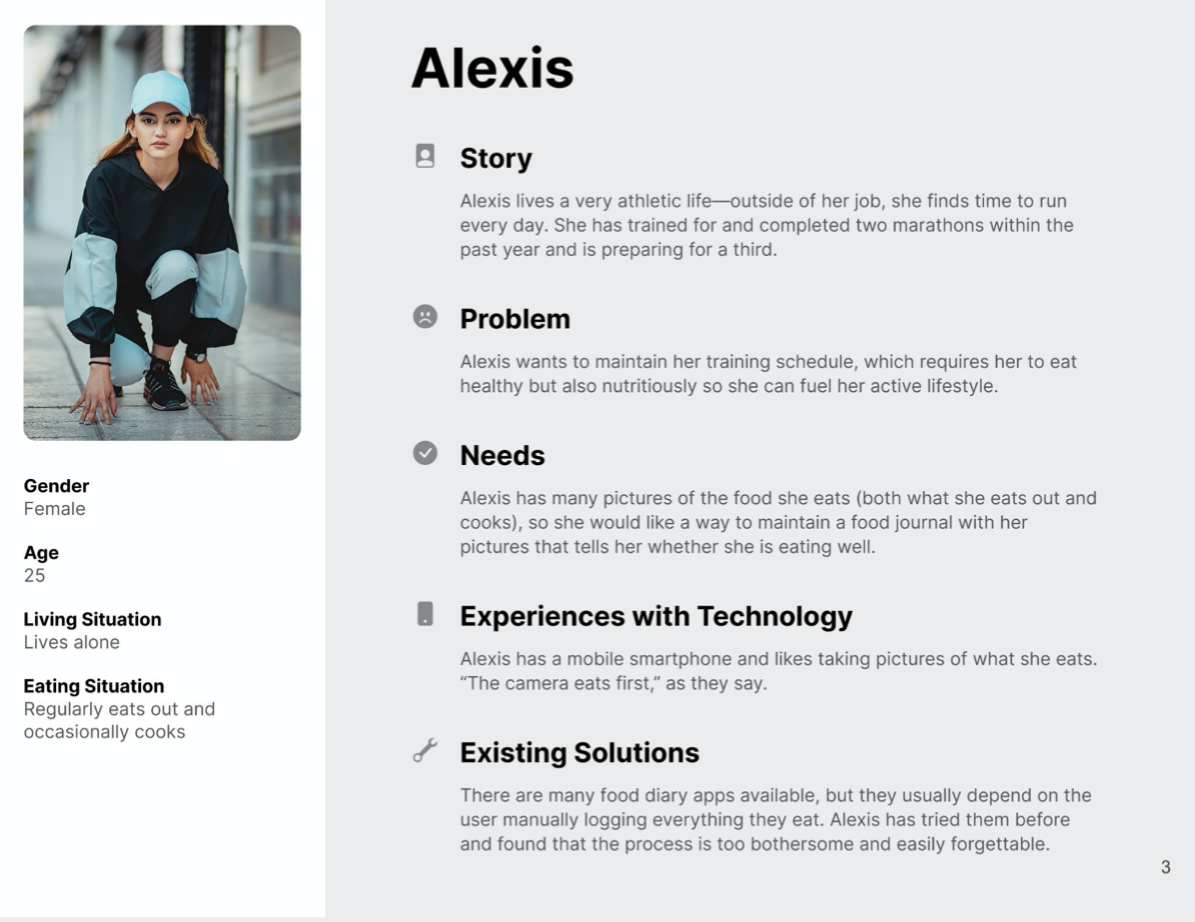}
    \end{subfigure}
     \begin{subfigure}[h]{0.49\textwidth}
        \centering
        \includegraphics[height=0.6\textwidth]{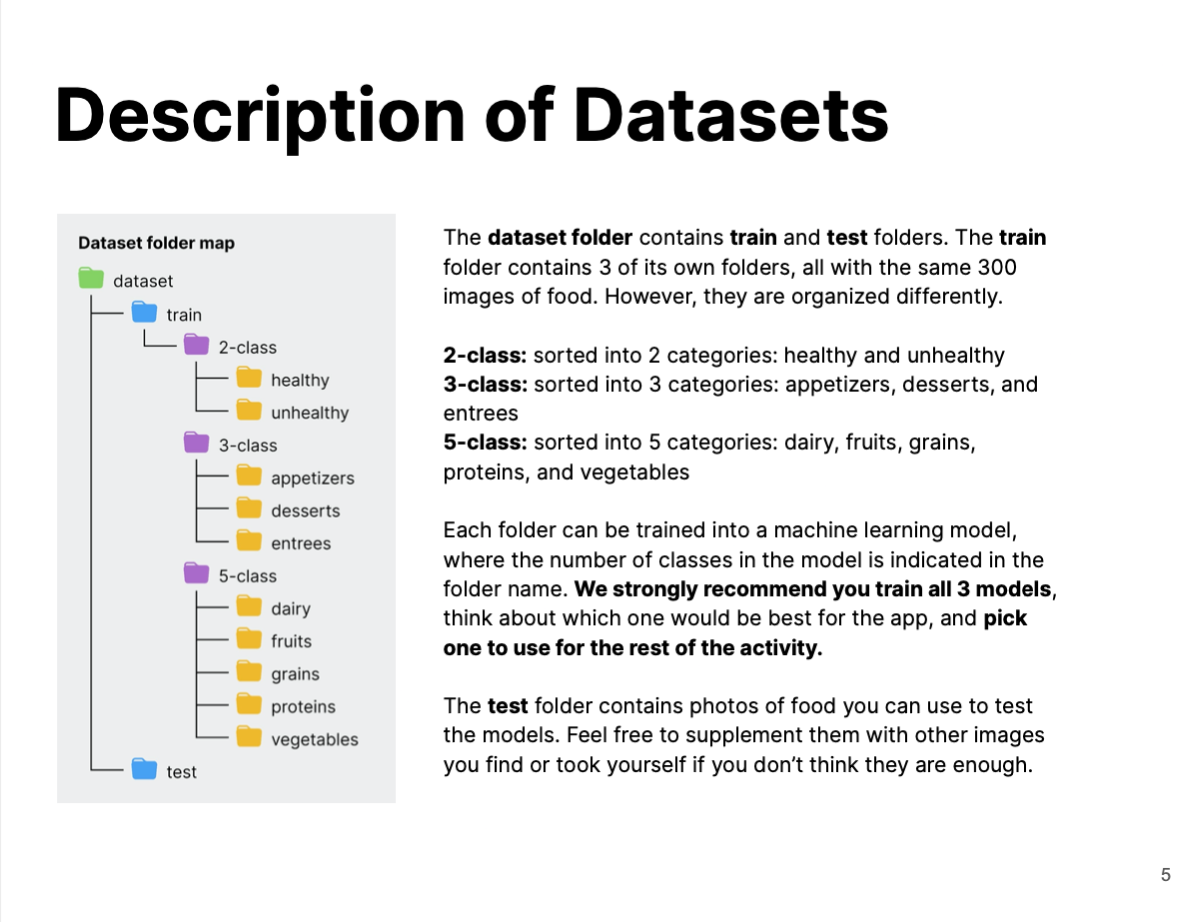}
    \end{subfigure}
     \begin{subfigure}[h]{0.49\textwidth}
        \centering
        \includegraphics[height=0.6\textwidth]{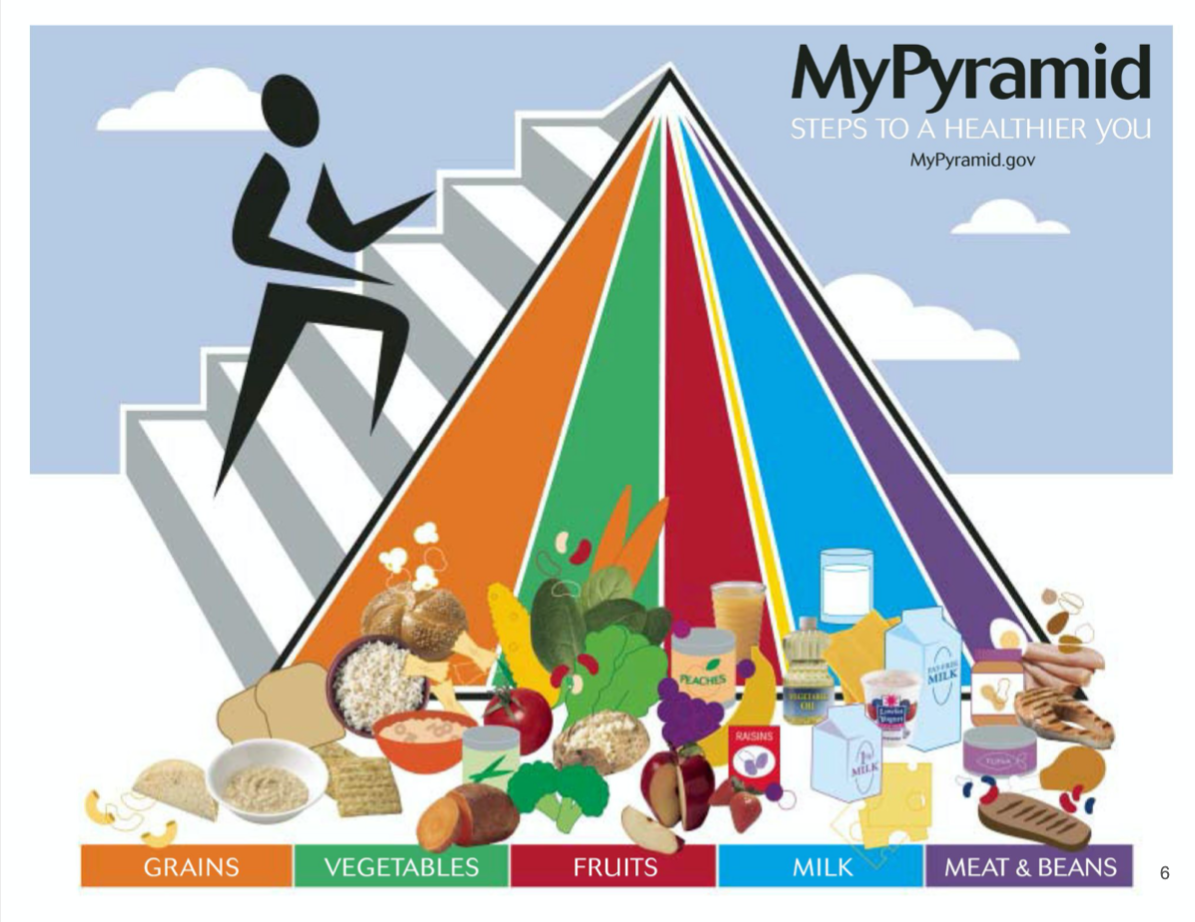}
    \end{subfigure}
     \begin{subfigure}[h]{0.49\textwidth}
        \centering
        \includegraphics[height=0.6\textwidth]{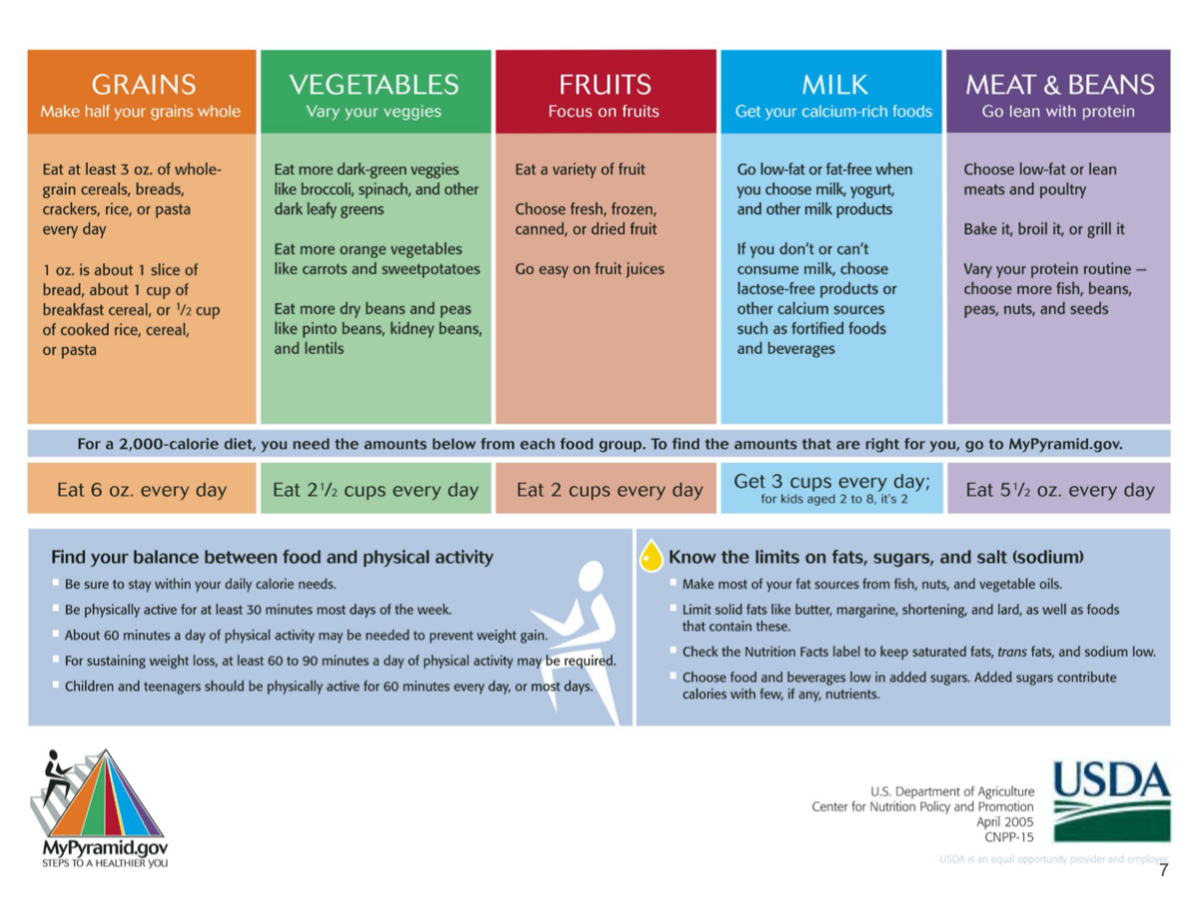}
    \end{subfigure}
     \begin{subfigure}[h]{0.49\textwidth}
        \centering
        \includegraphics[height=0.6\textwidth]{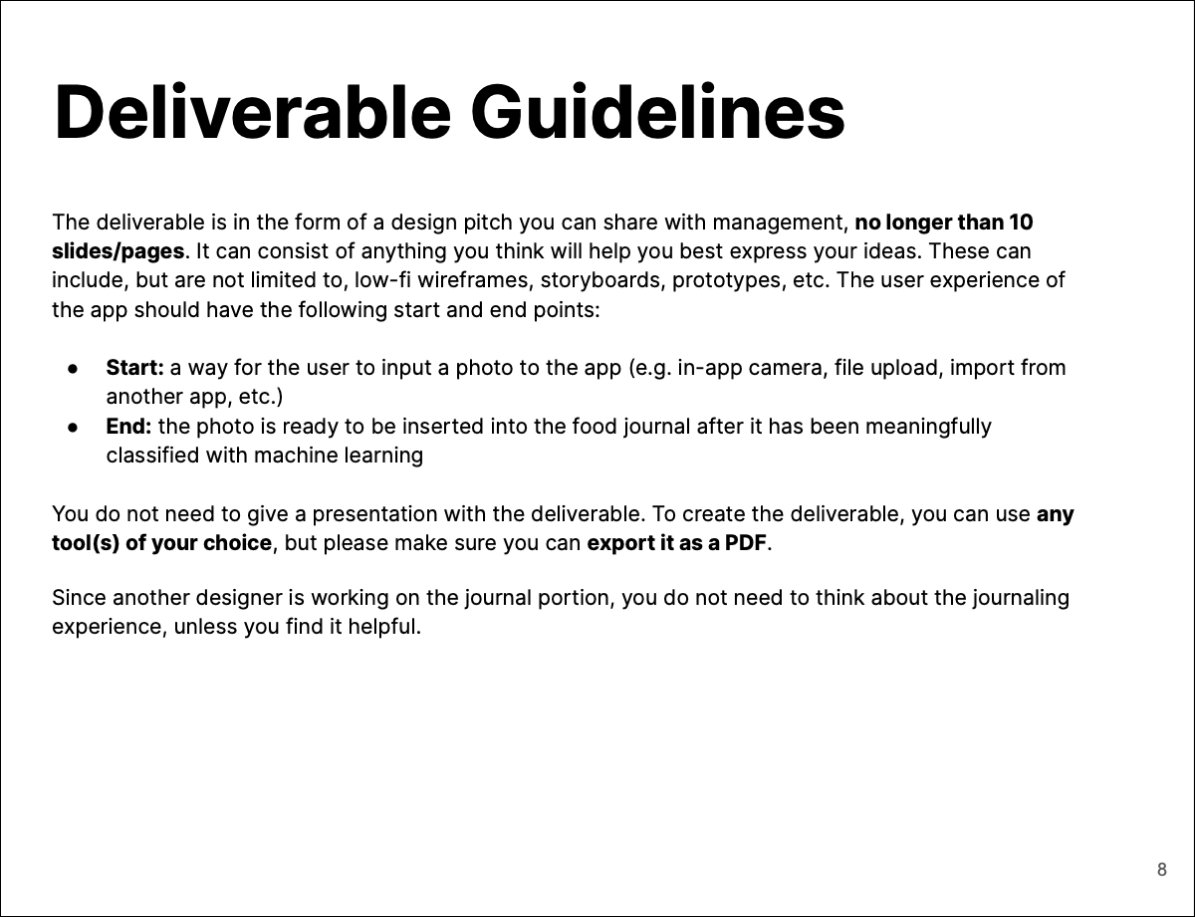}
    \end{subfigure}
    
    \caption{Pages from the instructional PDF file participants received. Note that participants received \textit{either} the female or male persona.}
    \label{f:top-tools}
\end{figure}
